# Supplementary material for: Latent Modulated Function for Computational Optimal Continuous Image Representation
Source: arXiv:2404.16451 source file (2024-04-25)
Supplement: Supplementary file 1 [file X_suppl.tex]

\clearpage
\setcounter{page}{1}
\maketitlesupplementary

\begin{table*}[ht]
\centering
%\small
\footnotesize
\caption{The network architectures of LMF-based ASSR methods and the reference methods. $^{*}$ indicates the use of latent modulations.}
\label{tab:detailed-network-architectures}
\begin{tabular}{l|c|c|c|c}
\hline
\multirow{2}{*}{Decoder} & \multirow{2}{*}{Params} & Latent & \multirow{2}{*}{Latent space} & \multirow{2}{*}{Render space} \bigstrut[t]\\
 & & modulation & & \bigstrut[t]\\
\hline

LIIF & 355K & $\times$ & $\times$ & $MLP=[580\times256, 3\times(256\times256), 256\times3]$ \bigstrut[t]\\
\cline{2-5}
LM-LIIF & 170K & $192$ & $MLP_{l}=[578\times208, 208\times208]$ & $MLP_{r}=[20\times16^{*}, 5\times(16\times16^{*}), 16\times3]$ \bigstrut[t]\\
\hline

LTE & 506K & $\times$ & \makecell{$Conv_{freq}=[64\times256], ks3$, \\$Conv_{coef}=[64\times256], ks3$, \\ $MLP_{phase}=[2\times128]$} & $MLP_{r}=[256\times256, 2\times(256\times256), 256\times3]$ \bigstrut[t]\\
\cline{2-5}
LM-LTE & 278K & $256$ & \makecell{$Conv_{freq}=[64\times128], ks3$, \\$Conv_{coef}=[64\times128], ks3$, \\ $MLP_{phase1}=[2\times64]$, \\$MLP_{l}=[128\times288, 288\times288]$} & \makecell{$MLP_{phase2}=[2\times8],$ \\ $MLP_{r}=[16\times16^{*}, 7\times(16\times16^{*}), 16\times3]$} \bigstrut[t]\\
\hline

CiaoSR-1.4M & 1.429M & $\times$ & \textcolor{black}{Non-local attention module} & \makecell{$MLP_{k}=[580\times256, 3\times(256\times256), 256\times576]$, \\$MLP_{v}=[644\times256, 3\times(256\times256), 256\times640]$, \\$MLP_{q}=[640\times256, 3\times(256\times256), 256\times3]$} \bigstrut[t]\\
\cline{2-5}
CiaoSR-3.1M & 3.065M & $\times$ & \textcolor{black}{Non-local attention module} & \makecell{$MLP_{k}=[1624\times256, 3\times(256\times256), 256\times1620]$, \\$MLP_{v}=[1804\times256, 3\times(256\times256), 1800\times3]$, \\$MLP_{q}=[1800\times256, 3\times(256\times256), 256\times3]$} \bigstrut[t]\\

\cline{2-5}
LM-CiaoSR & 753K & $256$ & \makecell{\textcolor{black}{Non-local attention module,} \\$MLP_{k}=[260\times256, 256\times256]$, \\$MLP_{v}=[324\times256, 256\times320]$, \\$MLP_{q}=[576\times256, 256\times256]$, \\$MLP_{l}=[320\times288, 288\times288]$} & $MLP_{r}=[34\times16^{*}, 7\times(16\times16^{*}), 16\times3]$ \bigstrut[t]\\
\hline

\end{tabular}
\end{table*}

We organize our supplementary material as follows. In Section \ref{section:suppl-1}, we provide additional implementation details and comprehensive network architectures for our proposed LMF-based ASSR methods. In Section \ref{section:suppl-2}, we conduct an in-depth efficiency analysis of LMF-based ASSR methods and the original ASSR methods. Section \ref{section:suppl-3} showcases the effectiveness of CMSR by providing additional details and results. Finally, Section \ref{section:suppl-4} delves into more visual results for various ASSR scenarios.

\section{More Implementation Details}
\label{section:suppl-1}
In Table \ref{tab:detailed-network-architectures}, we present the detailed network structures of our LMF-based ASSR methods, namely LM-LIIF, LM-LTE, and LM-CiaoSR. For reference, we also provide the network architectures of the original INR-based ASSR methods, namely LIIF \cite{chen2021learning}, LTE \cite{lee2022local}, and CiaoSR \cite{cao2023ciaosr}. In the table, the notation $MLP=[580 \times 256, 3 \times (256 \times 256), 256 \times 3]$ represents an MLP architecture. Firstly, it includes an input linear layer with input and output dimensions of 580 and 256, respectively. Additionally, there are three hidden linear layers, each with both input and output dimensions of 256. Finally, there is an output linear layer with input and output dimensions of 256 and 3, respectively. Regarding the activation function, we utilize the ReLU activation after every linear layer, except for the output linear layer in the MLP, which does not use any activation function. The notation $Conv=[64\times256], ks=3$ represents a convolutional layer with input and output features of 64 and 256 dimensions, respectively, and a kernel size of 3.

%LIIF employs a 5-layer MLP with 256 dimensions in HR-HD space, while LM-LIIF employs a 2-layer latent MLP with 192 dimensions in LR-HD space, and a 7-layer render MLP with 16 dimensions in HR-LD space. 
%\textcolor{cyan}{As for LM-LTE, we employ a 2-layer latent MLP with 256 dimensions, a 9-layer render MLP with 16 dimensions, and a local texture estimator \cite{lee2022local} with 128 dimensions.} 
%\textcolor{cyan}{LM-CiaoSR employs four 2-layer latent MLPs with 256 dimensions to generate key, value, and query information, followed by a 9-layer render MLP with 16 dimensions.}

Local ensemble is proposed in LIIF \cite{chen2021learning}, which ensures continuous prediction by merging the four predictions from the top-left, top-right, bottom-left, and bottom-right latent codes. Both our LMF-based ASSR methods and the reference methods utilize local ensemble in HR space:
\begin{equation}
  I(x^{*}_{i, j}) = \sum_{t \in \{tl, tr, bl, br\}} \frac{A(v^{*}_{t'}, x^{*}_{i, j})}{A_{R^{*}}} f_{\theta_{r}, m^{*}_{t'}}(z^{*}_{t'}, x^{*}_{i, j}),
  \label{con:local-ensemble}
\end{equation}
where $x^{*}_{i, j}$ is any query coordinate closest to $z^{*}$, and $v^{*}_{t}$ is the coordinate of $z_{t}^{*}$. $z^{*}_{t}$ is one of the latent codes at the top-left ($tl$), top-right ($tr$), bottom-left ($bl$), bottom-right ($br$) corners center around $z^{*}$. $A(v^{*}_{t'}, x^{*}_{i, j})$ refers to the area of the rectangle between the coordinates $v^{*}_{t'}$ and $x^{*}_{i, j}$, where $t'$ is diagonally opposite to $t$ (\ie, (1,1) to (-1,-1), (-1,1) to (1,-1)). $A_{R^{*}}$ represents the area of the rectangle $R^{*}$ whose vertices are $\{tl, tr, bl, br\}$. 

LIIF also introduces feature unfolding \cite{chen2021learning}, which concatenates the nearby $3\times3$ feature vectors as the latent code:
\begin{equation}
  z^{*} = Concat(\{z^{*}_{k, l}\}_{k, l \in \{-1,0,1\}}),
  \label{con:feature-unfolding}
\end{equation}
where $z^{*}_{k, l}$ is one of the $3\times3$ feature vectors center around the latent code $z^{*}$. Both LIIF and CiaoSR require the use of $3\times3$ feature unfolding in HR space, while LM-LIIF and LM-CiaoSR only require $3\times3$ and $2\times2$ feature unfolding in latent space, respectively. In contrast, both LTE and LM-LTE replace the feature unfolding strategy with the Local Texture Estimator \cite{lee2022local}, This estimator consists of a frequency convolutional layer, a coefficient convolutional layer, and an MLP for phase.

\section{Efficiency Analysis}
\label{section:suppl-2}
In this section, we present the computational analysis of LIIF and LM-LIIF. These two methods are representative as they focus on the fundamentals of continuous image representation. We analyze upsampling an $h\cdot w\cdot 3$ input image with a scale factor $s$. Before decoding, the encoder generates $h\cdot w\cdot 64$ feature maps using the input image. To quantify the computational complexity of LIIF, we can formulate it as the number of multiplications used by LIIF:
\begin{equation}
\begin{split}
  Mul_{\text{LIIF}}&=4 (d_{in} d_{h} + (k - 2) d_{h}^{2} + d_{h} d_{out}) s^{2} h w \\
  %&=4((576+4)*256+3*256*256+3*256)*s^{2}\cdot h\cdot w, \\
  &=1383424 s^{2} h w,
  \label{con:computation-liif}
\end{split}
\end{equation}
where $d_{in}=580$ denotes the dimension of the MLP input, which consists of coordinates, cells, and the latent code using $3\times3$ feature unfolding. $d_{h}=256$ represents the hidden dimension of the decoding MLP, while $d_{out}=3$ represents the dimension of the output pixel value. The depth of the decoding MLP is denoted by $k=5$.

To accomplish the same upsampling task, the number of multiplications used by LM-LIIF can be formulated as:
\begin{equation}
\begin{split}
  Mul_{\text{LM-LIIF}}= &(d_{in} d_{l} + (k_{l} - 1) d_{l}^{2}) h w + \\
  & 4 (d_{c} d_{r} + (k_{r} - 2) d_{r}^{2} + d_{r} d_{out}) s^{2} h w \\
  =&163488 h w + 6592 s^{2} h w,
  \label{con:computation-lm-liif}
\end{split}
\end{equation}
where $d_{in}=578$ represents the dimension of the latent MLP input, which consists of cells and the latent code using $3\times3$ feature unfolding. $d_{c}=20$ represents the dimension of the render MLP input, which consists of the compressed latent code, coordinates, and cells. The hidden dimension of the latent MLP and the render MLP are denoted by $d_{l}=208$ and $d_{r}=16$, respectively. The depth of the latent MLP and the render MLP are represented by $k_{l}=2$ and $k_{r}=7$, respectively.

Compare Eq. \ref{con:computation-liif} and Eq. \ref{con:computation-lm-liif}, it becomes apparent that our LM-LIIF requires significantly fewer multiplications than LIIF, and the reduction in multiplications $Mul_{\text{LIIF}} - Mul_{\text{LM-LIIF}}$ increases as the scale factor increases. For large scales, most of the multiplications in LM-LIIF are attributed to the latent MLP, which remains unaffected by the scale factor. Even for identity mapping ($\times 1$ SR), our LM-LIIF reduces the number of multiplications by over $87.7\%$.

%\textcolor{cyan}{In Table \ref{}}, we further evaluate the computational cost of each component in our LMF-based methods and the reference methods. Specifically, we divide the decoding process into latent code preparing, shared latent decoding, and rendering. \textcolor{cyan}{For LTE and LM-LTE, the Local Texture Estimator is identified as latent code preparing. For CiaoSR and LM-CiaoSR, generating the non-local attention is identified as latent code preparing. As shown in the Table, the computational cost of our LMF-based methods is focused on the latent code preparing and shared latent decoding, which remains unchanged as the scale factor increases. Moreover, we maintain the same latent code preparing process to align with the reference methods, thereby causing inevitable computational cost for LM-CiaoSR on every tested scales.}

\begin{figure}[t]
  \centering
  \includegraphics[width=\linewidth]{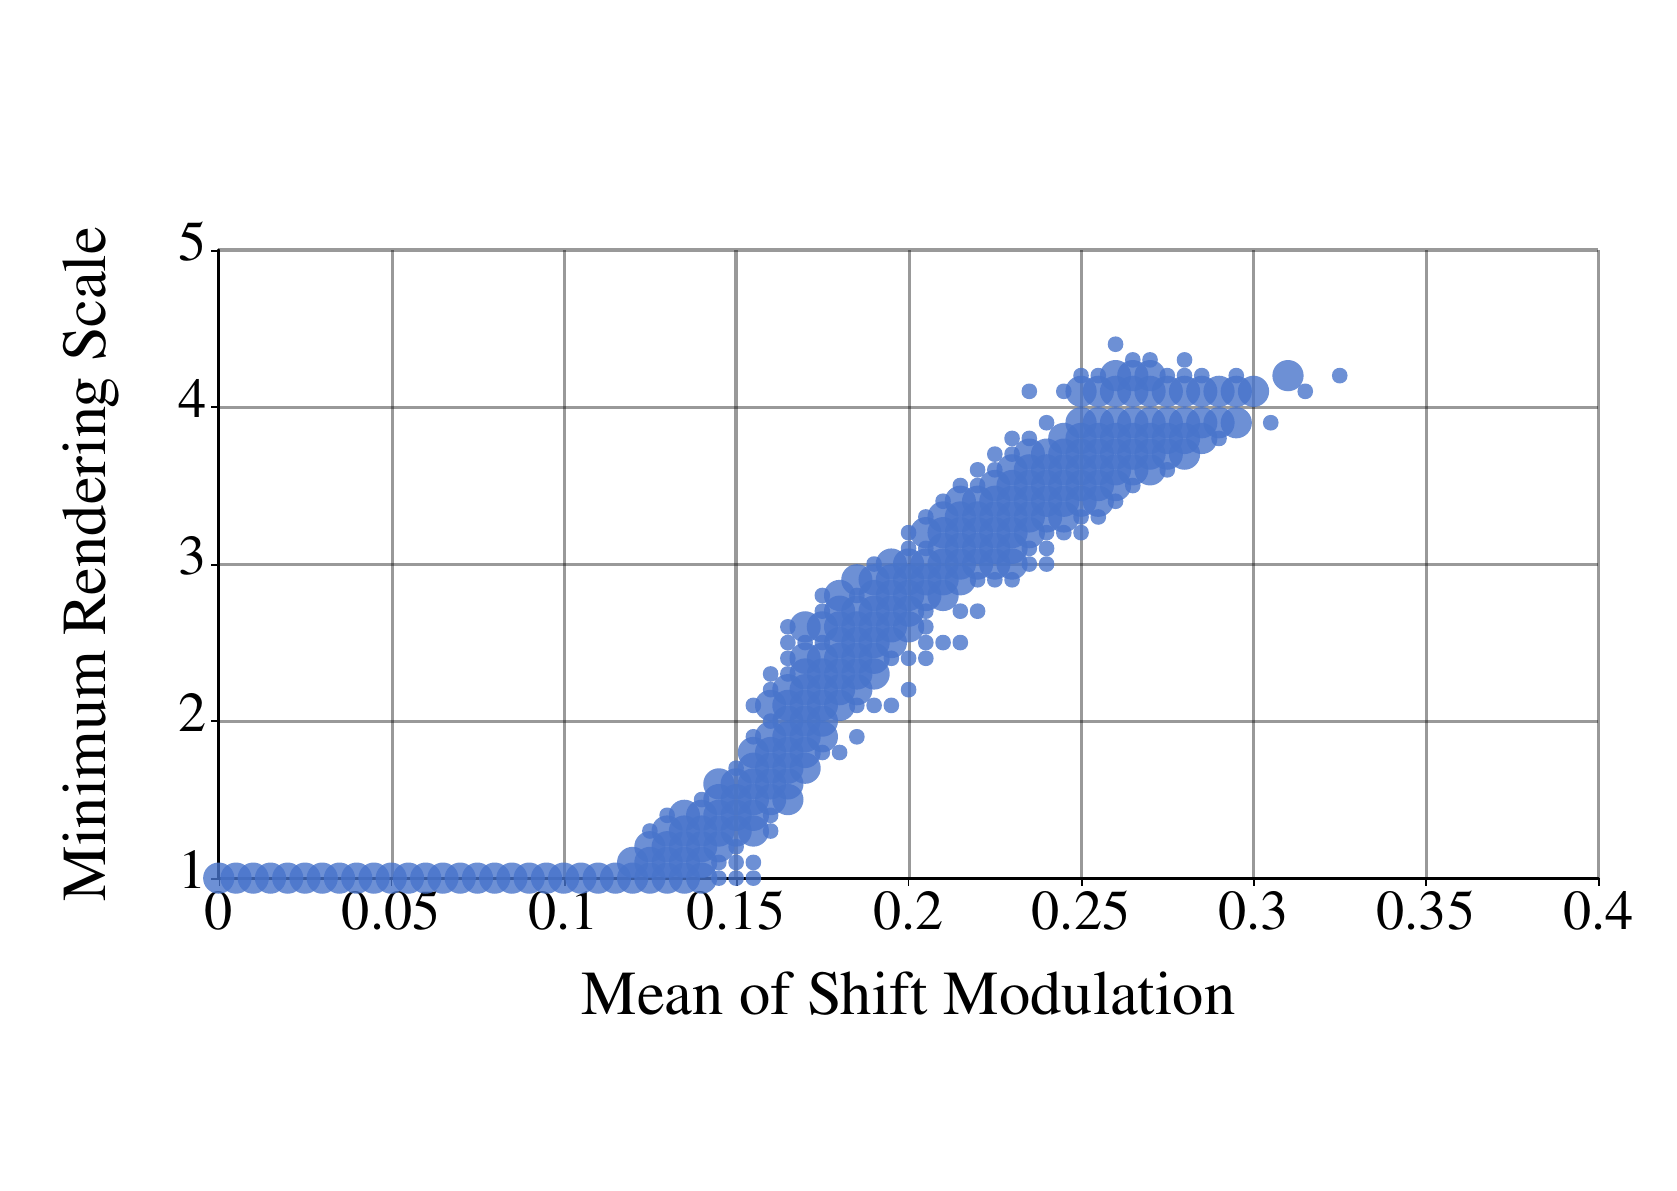}
  \caption{The positive correlation between the means of shift modulation and the minimum rendering scale factors in LM-LTE.}
  %\Description{}
  \label{fig:mod-scale-relation-lm-lte}
\end{figure}

\begin{figure}[t]
  \centering
  \includegraphics[width=\linewidth]{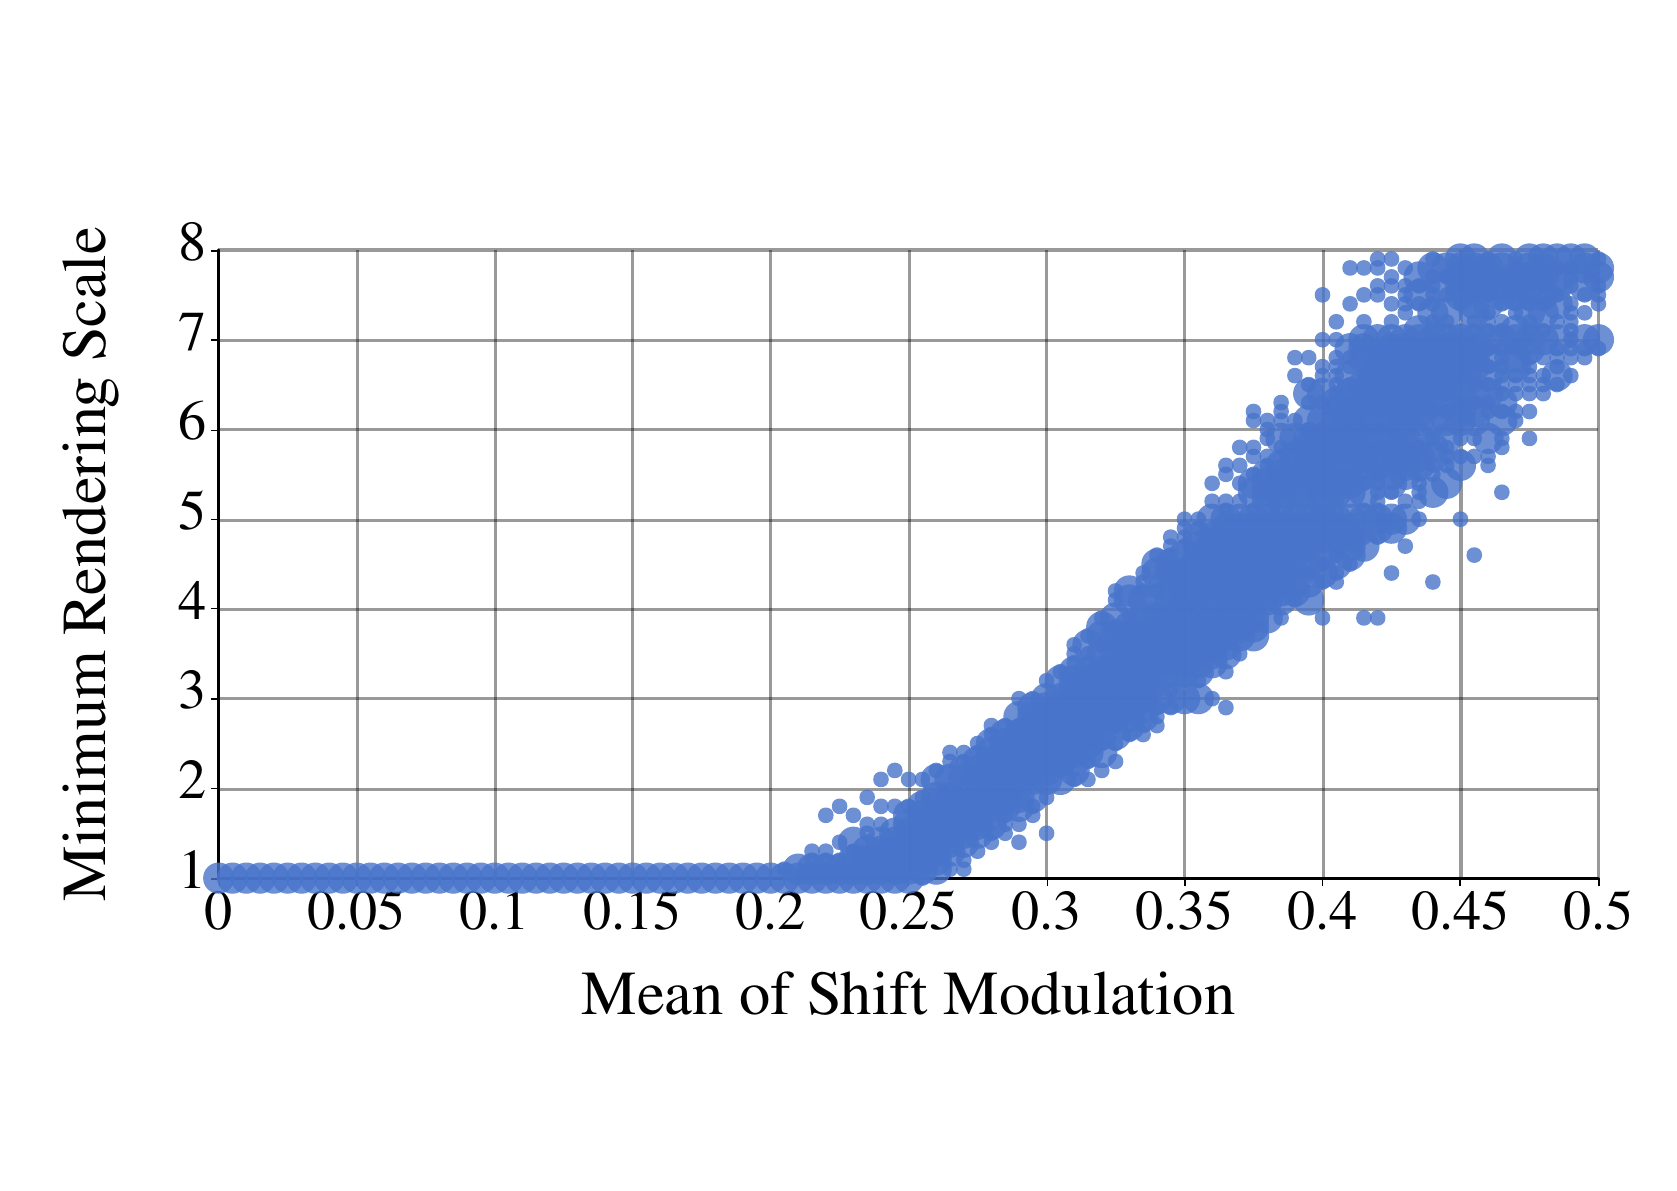}
  \caption{The positive correlation between the means of shift modulation and the minimum rendering scale factors in LM-CiaoSR.}
  %\Description{}
  \label{fig:mod-scale-relation-lm-ciaosr}
\end{figure}

\section{Details and Results on CMSR}
\label{section:suppl-3}
In Figures \ref{fig:mod-scale-relation-lm-lte} and \ref{fig:mod-scale-relation-lm-ciaosr}, we visualize the positive correlation between the means of shift modulation and the minimum rendering scale factors in two different methods, LM-LTE and LM-CiaoSR. Specifically, we uniformly sample 100 means of shift modulation from the range of $[0, 0.5]$ and measure their corresponding minimum scale factors using the LR images from the training set. The results clearly indicate a positive correlation between the means of shift modulation and the minimum scale factors in both LM-LTE and LM-CiaoSR methods. An intriguing observation is that the minimum scale factors in LM-CiaoSR are relatively larger than those in LM-LTE, suggesting superior SR performance and generalization of LM-CiaoSR over LM-LTE. These results provide valuable and comprehensive insights into the effectiveness of latent modulation and the underlying mechanisms and performance characteristics of INR-based ASSR methods. %the relationship between means of shift modulation and minimum scale factors. %, contributing to a deeper understanding of the underlying mechanisms and performance characteristics of the LM-LTE and LM-CiaoSR methods.

\begin{algorithm}
\caption{Creating Scale2Mods table for LMF}
\label{alg:Scale2Mods-table}
\SetKwInOut{Input}{Input}
\SetKwInOut{Output}{Output}
\Input{LR images $\{I_{0}, \dots, I_{J}\}$, MSE threshold $\tau$, common scale factors $\{s_{0}, \dots, s_{K}\}$, means of shift modulation $\{0, u, 2u, \dots, 1\}$ sampled with interval $u$}
\Output{Scale2Mods table $T_{\tau}=\{s_{0}: [m^{s_{0}}_{min}, m^{s_{0}}_{max}], \dots, s_{K}: [m^{s_{K}}_{min}, m^{s_{K}}_{max}]\}$}
\For{$I_{j} \in \{I_{0}, \dots, I_{J}\}$}{
$I^{s_{K}}_{j}=LMF_{s_{K}}(I_{_{j}})$\;
\textcolor{black}{Compute means of shift modulation $M_{j}$ for $I_{j}$}\;
\For{$s_{k} \in \{s_{0}, \dots, s_{K}\}$}{
    %Render $I_{i}$ with scale $s_{j}$ using LMF\;
    %Upsample $I_{i}^{s_{j}}$ with scale $\frac{s_{max}}{s_{j}}$ using bilinear interpolation\;
    $I^{s_{K}'}_{j}=Bilinear_{ \frac{s_{K}}{s_{k}} }( LMF_{s_{k}}(I_{_{j}}) )$\;
    $[m^{s_{k}}_{min}, m^{s_{k}}_{max}]=T_{\tau}(s_{k})$\;
    \For{$m_{l} \in \{0, u, 2u, \dots, 1\}$}{
        \textcolor{black}{Create a filter $Filter(I): m_{l} - \frac{u}{2} \le M \le m_{l} + \frac{u}{2}$}\;
        $Error_{k, l}=MSE(Filter(I_{j}^{s_{K}}), Filter(I^{s_{K}'}_{j}))$\;
        \eIf{$Error_{k, l} \le \tau$}{
            $m^{s_{k}}_{max}=Min(m^{s_{k}}_{max}, m_{l})$\;
            $m^{s_{k+1}}_{min}=m^{s_{k}}_{max}$\;
        }{
            break\;
        }
        $T_{\tau}(s_{k})=[m^{s_{k}}_{min}, m^{s_{k}}_{max}]$\;
    }
}
}
\Return $T_{\tau}$\;
\end{algorithm}

\begin{algorithm}
\caption{Controllable Multi-Scale Rendering}
\label{alg:cmsr}
\SetKwInOut{Input}{Input}
\SetKwInOut{Output}{Output}
\Input{LR image $I_{LR}$, target scale factor $s_{target}$, Scale2Mods table $T=\{s_{0}: [m^{s_{0}}_{min}, m^{s_{0}}_{max}], \dots, s_{K}: [m^{s_{K}}_{min}, m^{s_{K}}_{max}]\}$}
\Output{SR image $I_{SR}$}
\textcolor{black}{Compute means of shift modulation $M_{LR}$ for $I_{LR}$}\;
Initialize $s_{-1}=1, I_{s_{-1}}=I_{LR}$\;
\For{$s_{k} \in \{s_{0}, \dots, s_{K}\}$}{
    \If{$s_{k} > s_{target}$}{
        $I_{SR}=Bilinear_{\frac{s_{target}}{s_{k-1}}}(I_{s_{k-1}})$\;
        \textcolor{black}{Create a filter $Filter(I): M \ge m^{s_{k-1}}_{max}$}\;
        $Filter(I_{SR})=Render_{s_{target}}(Filter(I_{LR}))$\;
        break\;
    }
    $I_{s_{k}}=Bilinear_{\frac{s_{k}}{s_{k-1}}}(I_{s_{k-1}})$\;
    %Upsample $I_{s_{i-1}}$ with scale $\frac{s_{i}}{s_{-1}}$ using bilinear interpolation\;
    %Query T to obtain $[m^{s_{i}}_{min}, m^{s_{i}}_{max}]$\;
    $[m^{s_{k}}_{min}, m^{s_{k}}_{max}] = T(s_{k})$\;
    \textcolor{black}{Create a filter $Filter(I): m^{s_{k}}_{min} \le M \le m^{s_{k}}_{max}$}\;
    % Create a filter for pixel whose mean of shift modulation $m \in M_{LR}$ satisfies
    $Filter(I_{s_{k}})=Render_{s_{k}}(Filter(I_{LR}))$\;
    \If{\textcolor{black}{$\forall m \in M_{LR}, m <= m^{s_{k}}_{max}$}}{
        $I_{SR}=Bilinear_{\frac{s_{target}}{s_{k}}}(I_{s_{k}})$\;
        break\;
    }
}
\Return $I_{SR}$\;
\end{algorithm}

In Algorithm \ref{alg:Scale2Mods-table}, we present the detailed algorithm for creating the Scale2Mod table, denoted as $T_{\tau}=\{s_{0}: [m^{s_{0}}_{min}, m^{s_{0}}_{max}], \dots, s_{K}: [m^{s_{K}}_{min}, m^{s_{K}}_{max}]\}$. The purpose of this table $T_{\tau}$ is to map a given scale factor $s_{k}$ to the range of means of shift modulation $[m^{s_{k}}_{min}, m^{s_{k}}_{max}]$. For any input pixel whose mean of shift modulation $m$ satisfies $m^{s_{k}}_{min} \le m \le  m^{s_{k}}_{max}$, we render this pixel with its minimum scale factor $s_{k}$ by querying the table.
To create a Scale2Mod table with a specified MSE threshold $\tau$, we follow the steps outlined below. For each LR image $I_{j} \in \{I_{0}, \dots, I_{J}\}$ from the training set, we use LMF to render $I_{j}$ with the maximum scale $s_{K}$ to obtain the fully rendered image $I^{s_{K}}_{j}$. Also, we compute the means of shift modulation $M_{j}$ corresponding to $I_{j}$. %Given the LR image $I^{s_{K}}_{j}$, for each scale $s_{k} \in \{s_{0}, \dots, s_{K}\}$, we render $I_{j}$ with $s_{k}$ followed by bilinear interpolation with $\frac{s_{K}}{s_{k}}$. 
Next, for each scale factor $s_{k} \in \{s_{0}, \dots, s_{K}\}$ and each mean of shift modulation $m_{l} \in \{0, u, 2u, \dots, 1\}$, we calculate the MSE between the pixels in the fully rendered image $I^{s_{K}}_{j}$ and the pixels in the image rendered by LMF with $s_{k}$ followed by bilinear interpolation with $\frac{s_{K}}{s_{k}}$. Notably, we only compute the MSE for any pixel whose corresponding mean of shift modulation satisfies the condition $Abs(m - m_{l}) \le \frac{u}{2}$. If the MSE result is less than or equal to the MSE threshold $\tau$, we update the $m^{s_{k}}_{max}$ and $ m^{s_{k+1}}_{min}$ in $T_{\tau}$ using the current mean of shift modulation $m_{l}$. This process is repeated for each LR image in the training set, enabling us to create a generalized Scale2Mod table $T_{\tau}$. %The Scale2Mod table plays a crucial role in determining the appropriate minimum scale factor for each pixel, based on its corresponding mean of shift modulation.

In Algorithm \ref{alg:cmsr}, we demonstrate the detailed algorithm for CMSR. Given an LR image $I_{LR}$, a target upsampling scale factor $s_{target}$, and a Scale2Mods table $T_{\tau}$, we proceed as follows. Firstly, we compute the means of shift modulation $M_{LR}$ corresponding to $I_{LR}$, and initialize $s_{-1}$ as $1$, $I_{s_{-1}}$ as $I_{LR}$. For each scale factor $s_{k} \in \{s_{0}, \dots, s_{K}\}$, we check if $s_{k}$ is greater than $s_{target}$. If it is, we upsample the result from the last scale $s_{k-1}$ using bilinear interpolation with $\frac{s_{target}}{s_{k-1}}$. We then replace the unrendered pixels in this bilinear upsampled result with the corresponding pixels rendered with $s_{target}$. On the other hand, if $s_{k}$ is less than or equal to $s_{target}$, we upsample the last result $I_{s_{k-1}}$ using bilinear interpolation with $\frac{s_{k}}{s_{k-1}}$ to obtain the current result $I_{s_{k}}$. Next, we query the Scale2Mods table $T_{\tau}$ to obtain the range of means of shift modulation $[m^{s_{k}}_{min}, m^{s_{k}}_{max}]$. For the current scale $s_{i}$, we only need to render the pixels whose means of shift modulation fall within this range $[m^{i}_{min}, m^{i}_{max}]$. We repeat the above process iteratively until we obtain the final SR result or until all pixels have been rendered by LMF. This CMSR algorithm ensures that LMF takes into account the content-awareness of the LR image, allowing for effective and efficient SR with satisfactory visual quality.

\begin{figure*}[ht]
  \centering
  \includegraphics[width=\textwidth]{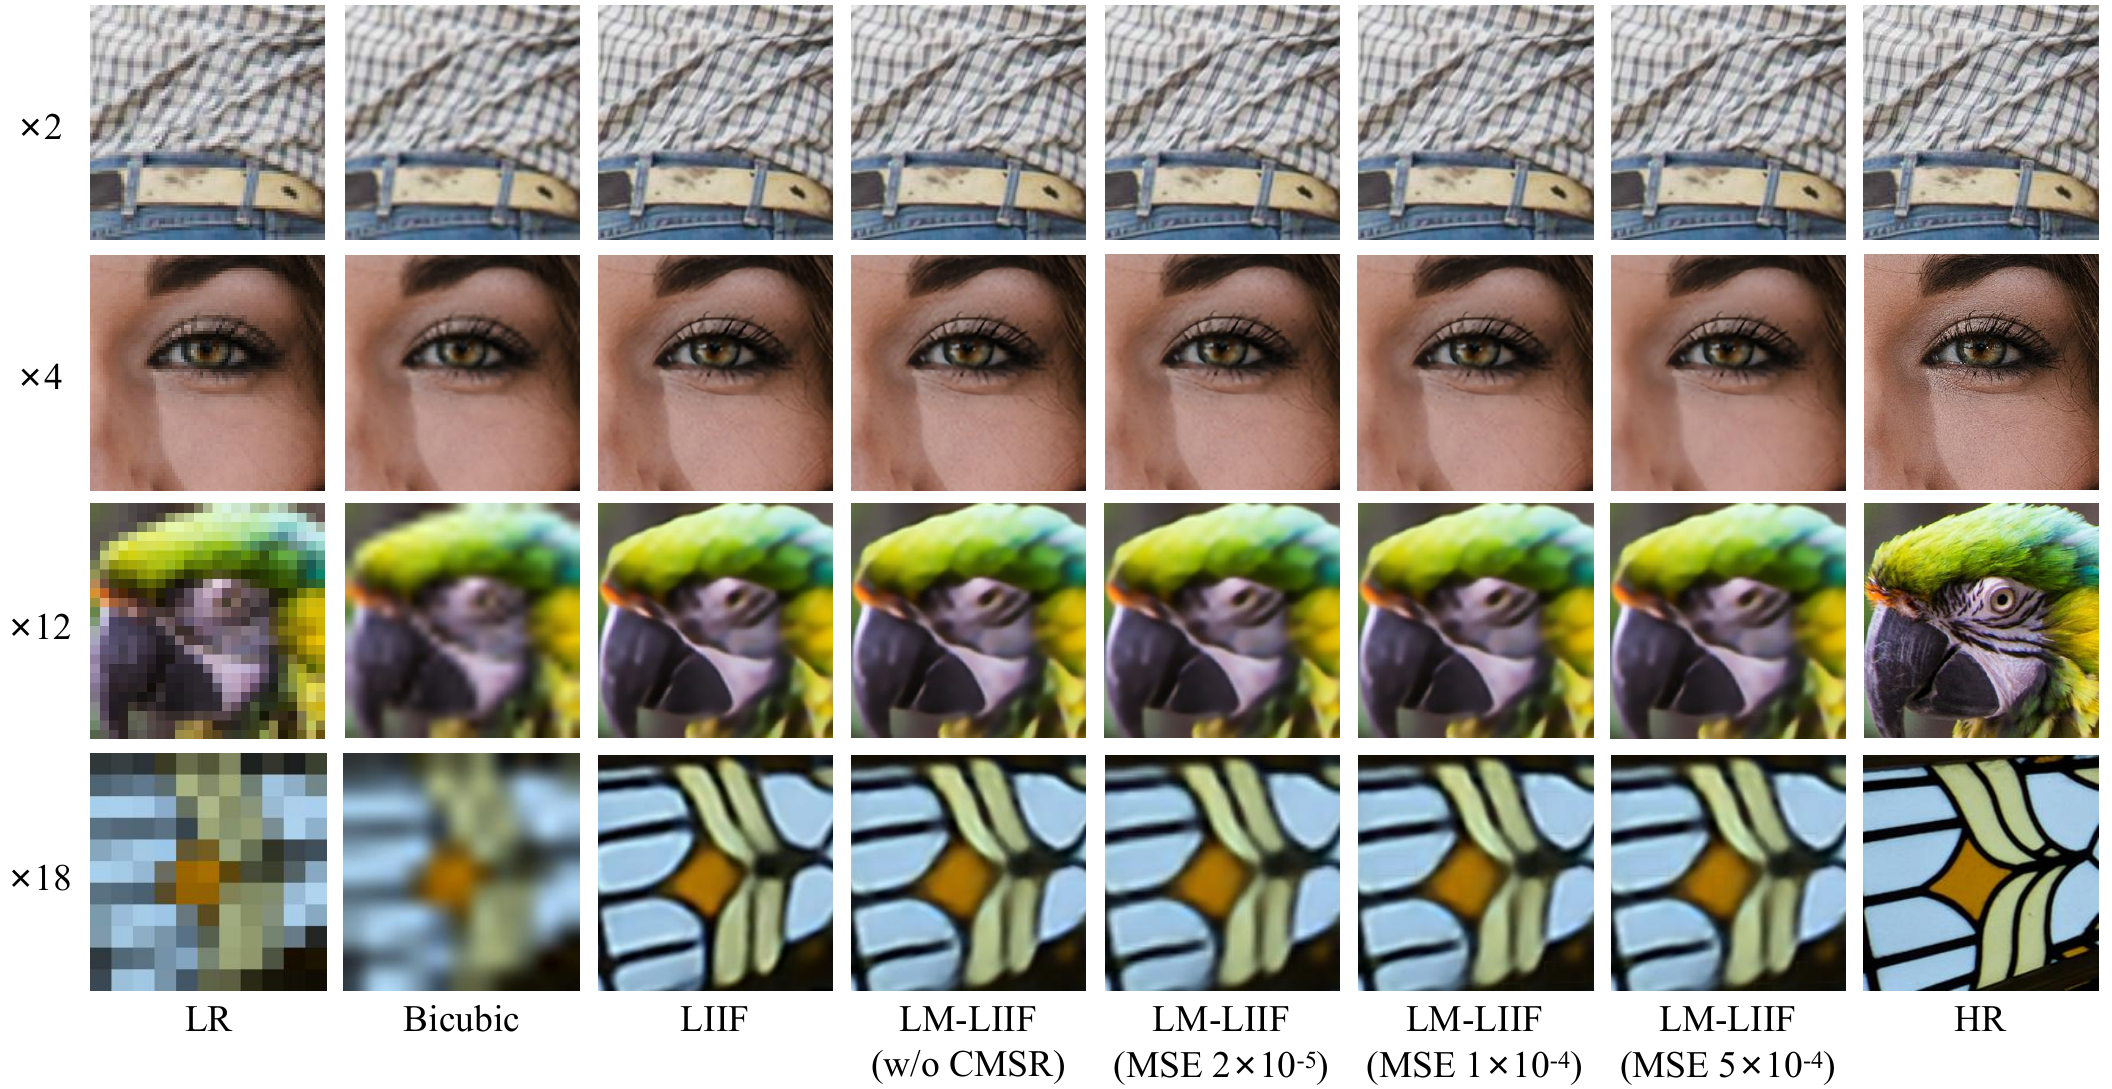}
  \caption{Qualitative comparison for using Scale2Mod tables with different MSE thresholds in CMSR. All of the ASSR methods use EDSR-b as the encoder.}
  %\Description{}
  \label{fig:cmsr_comparison}
\end{figure*}

\begin{table}[ht]
\centering
%\scriptsize
\caption{Ablation study (MACs results on DIV2K validation set) on the latent MLP and the render MLP with and w/o CMSR.}
\label{tab:components_efficiency}
\resizebox{\linewidth}{!}{
\begin{tabular}{l|c|c|cc|cc}
\hline
Method & Network & CMSR & $\times2$ & $\times4$ & $\times8$ & $\times16$ \bigstrut[t]\\
\hline

LIIF & Decoder & - & 3.567T & 3.567T & 3.567T & 3.567T \bigstrut[t]\\
LM-LIIF & Latent MLP & - & 107.92G & 26.98G & 6.73G & 1.67G \bigstrut[t]\\
%LM-LIIF & Latent MLP & - & 107.9154G & 26.9789G & 6.7305G & 1.6690G \bigstrut[t]\\

LM-LIIF & Render MLP & $\times$ & 17.41G & 17.41G & 17.37G & 17.23G \bigstrut[t]\\
%LM-LIIF & Decoder & $\times$ & 125.3204G & 44.3839G & 24.0990G & 18.8965G \bigstrut[t]\\

LM-LIIF & Render MLP & $\checkmark$ & 16.30G & 13.64G & 12.41G & 3.48G \bigstrut[t]\\
%LM-LIIF & Decoder & $\checkmark$ & 124.2175G & 40.6204G & 19.1382G & 5.1506G \bigstrut[t]\\
\hline

\end{tabular}
}
\end{table}

For an in-depth analysis of the computational savings afforded by CMSR, Table \ref{tab:components_efficiency} provides the MACs results on DIV2K validation set of the latent MLP and the render MLP with or without the final CMSR. EDSR-b \cite{lim2017enhanced} is utilized as the encoder. The results reveal that, particularly at scales 8 and 16, the computational cost is primarily attributable to the render MLP, and CMSR can significantly reduces the computations for the render MLP at these scales.

In Table \ref{tab:mean_of_shift_modulation}, we further investigate the effectiveness of using the means of shift modulation as the indicators of signal complexity. Here, we manually adjust the means of shift modulation by $\pm 0.2$ when used in CMSR. Utilizing EDSR-b \cite{lim2017enhanced} as the encoder and LM-LIIF as the decoder, the results validate that querying rendering scales based on precise means of shift modulation achieves an optimal balance between PSNR performance and computational efficiency.

\begin{table}[ht]
\centering
\caption{Ablation study (PSNR/MACs of the render MLP on DIV2K validation set) on the means of shift modulation (referred to as ``Mean'') in CMSR.
}
\label{tab:mean_of_shift_modulation}
\resizebox{\linewidth}{!}{
\begin{tabular}{l|c|cc|cc}
\hline
MSE thresh. & Query  & $\times2$ & $\times4$ & $\times8$ & $\times16$ \bigstrut[t]\\
\hline

$1 \times 10^{-4}$ & Mean & \makecell{34.62/ \\ \textbf{13.63G}} & \makecell{28.98/ \\ \textbf{11.71G}} & \makecell{25.39/ \\ \textbf{8.35G}} & \makecell{\textbf{22.62}/ \\ \textbf{2.50G}} \bigstrut[t]\\
$2 \times 10^{-5}$ & Mean - 0.2 & \makecell{34.53/ \\ 14.88G} & \makecell{28.98/ \\ 16.04G} & \makecell{\textbf{25.40}/ \\ 14.78G} & \makecell{\textbf{22.62}/ \\ 2.68G} \bigstrut[t]\\
$2 \times 10^{-5}$ & Mean + 0.2 & \makecell{\textbf{34.65}/ \\ 17.41G} & \makecell{\textbf{28.99}/ \\ 17.40G} & \makecell{\textbf{25.40}/ \\ 15.45G} & \makecell{\textbf{22.62}/ \\ 4.28G} \bigstrut[t]\\

$2 \times 10^{-5}$ & Mean & \makecell{\textbf{34.65}/ \\ 16.30G} & \makecell{\textbf{28.99}/ \\ 13.64G} & \makecell{\textbf{25.40}/ \\ 12.41G} & \makecell{\textbf{22.62}/ \\ 3.48G} \bigstrut[t]\\
\hline

\end{tabular}
}
\end{table}

In Figure \ref{fig:cmsr_comparison}, we present the qualitative comparison of using Scale2Mod tables at varying MSE thresholds in CMSR. Specifically, we experiment with thresholds at $2 \times 10^{-5}$, $1 \times 10^{-4}$, and $5 \times 10^{-4}$. All of the ASSR methods utilize EDSR-b \cite{lim2017enhanced} as the encoder, and our LMF-based ASSR methods utilize LM-LIIF as the decoder. As depicted in the figure, setting the MSE threshold of $2 \times 10^{-5}$ in CMSR yields the same visual quality as LM-LIIF without CMSR. Notably, further increasing the MSE thresholds to $1 \times 10^{-4}$ and $5 \times 10^{-4}$ maintains satisfactory visual quality while significantly reducing the computational cost.

\begin{figure*}[ht]
  \centering
  \includegraphics[width=\textwidth]{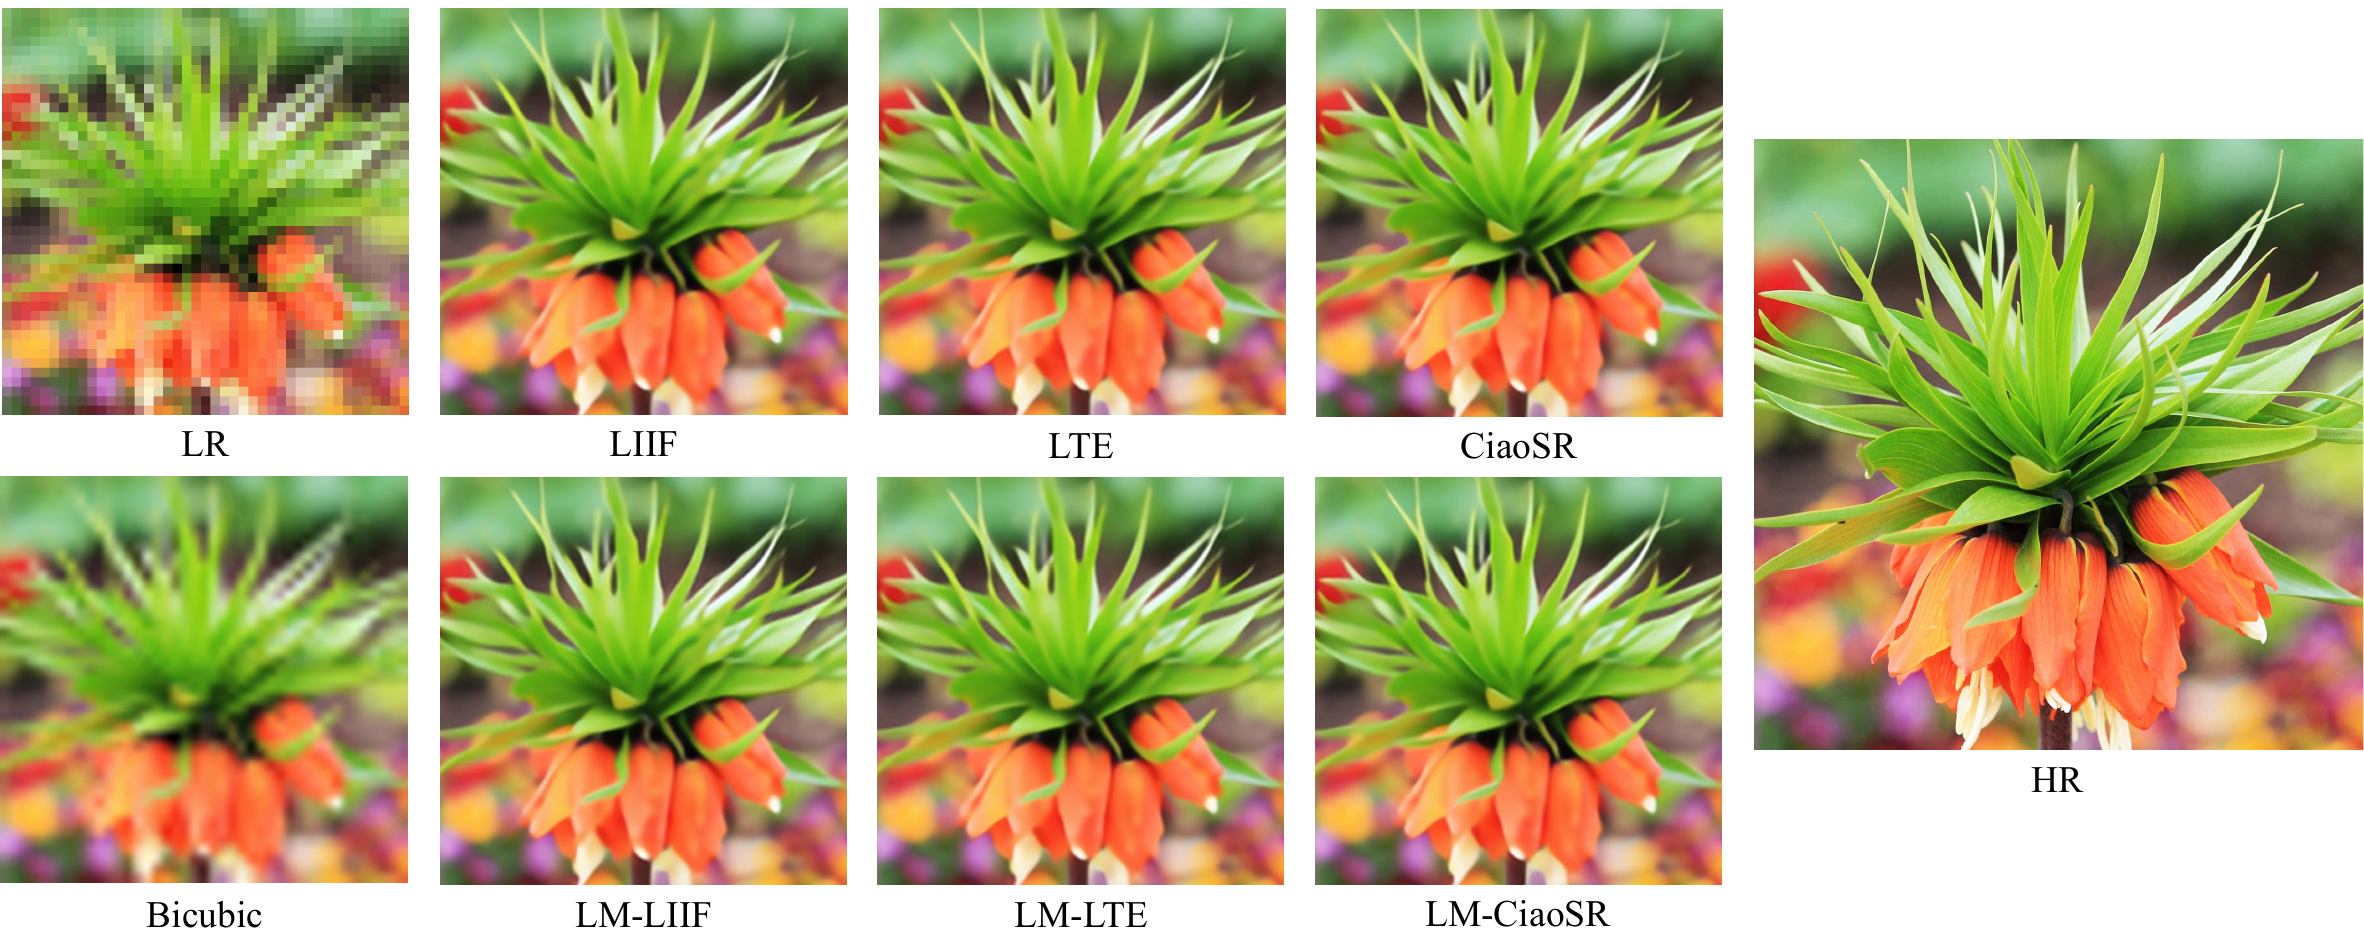}
  \caption{Qualitative comparison for $\times 30$ SR. All of the ASSR methods use SwinIR as the encoder.}
  %\Description{}
  \label{fig:extreme_large-scale_comparison}
\end{figure*}

\section{More Visual Results}
\label{section:suppl-4}
In this section, we demonstrate additional visual results obtained from test sets to showcase the effectiveness of our LMF-based ASSR methods. Figure \ref{fig:extreme_large-scale_comparison} illustrates the application of ASSR methods on the challenging task of extreme large-scale SR, specifically $\times 30$ SR. For all the ASSR methods showcased, SwinIR \cite{liang2021swinir} is used as the encoder. As depicted in the figure, LMF, as a continuous image representation, excels at producing sharp edges and realistic textures when dealing with such extreme scales, outperforming the bicubic interpolation method by a significant margin.

In Figure \ref{fig:qualitative_comparison_edsr-b} and Figure \ref{fig:qualitative_comparison_rdn}, we present additional qualitative comparisons for ASSR using EDSR-b \cite{lim2017enhanced} and RDN \cite{zhang2018residual} as the encoders, respectively. As illustrated in the figures, our LMF-based ASSR methods achieve visual quality comparable to that of the original ASSR methods in most cases, regardless of the encoder used.

%In Figure \ref{fig:non-integer-scale-comparison}, we show the visual comparison for text images with non-integer scale factors. All of the methods use SwinIR \cite{} as the encoder. \textcolor{cyan}{Compared to the reference INR-based ASSR methods, LMF-based methods is capable of restoring clearer texts with slightly fewer structural distortions, particularly the row 'multimedia', and the word 'your'.}

\begin{figure*}[ht]
  \centering
  \includegraphics[width=\textwidth]{author-kit-CVPR2024-v2/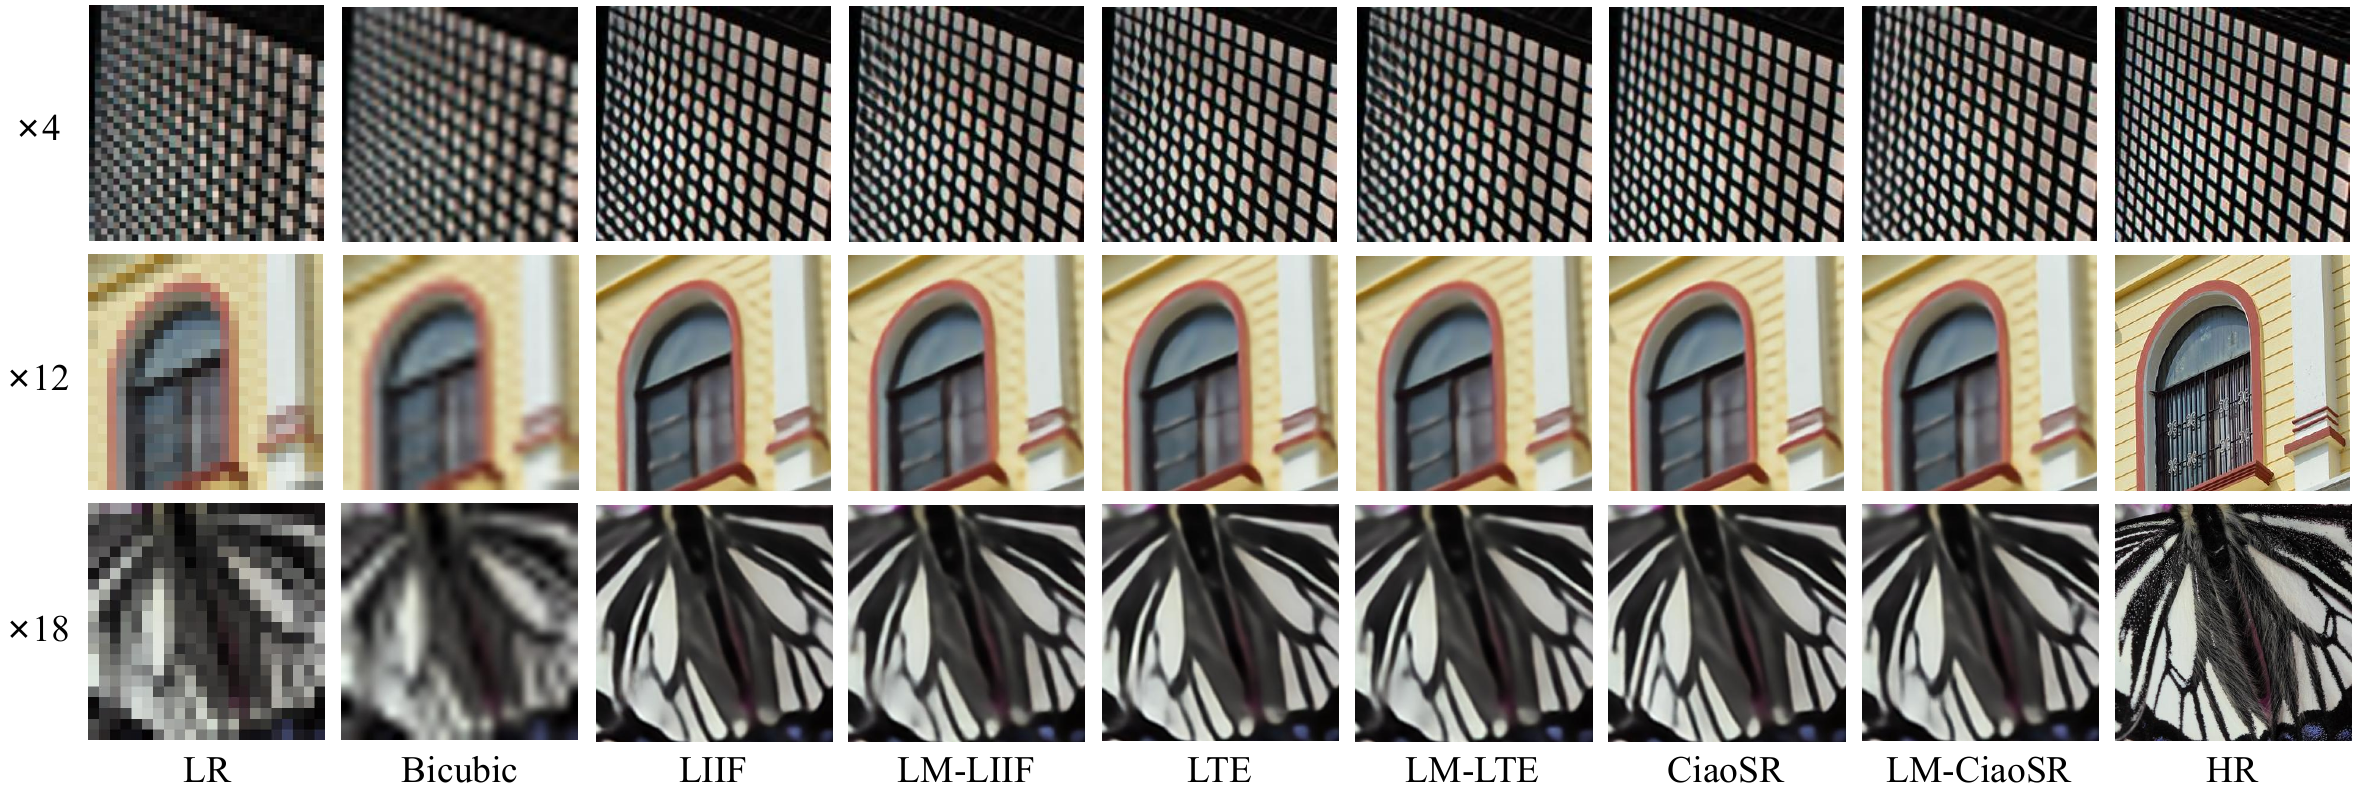}
  \caption{Qualitative comparison for ASSR. All of the ASSR methods use EDSR-b as the encoder.}
  %\Description{}
  \label{fig:qualitative_comparison_edsr-b}
\end{figure*}

\begin{figure*}[ht]
  \centering
  \includegraphics[width=\textwidth]{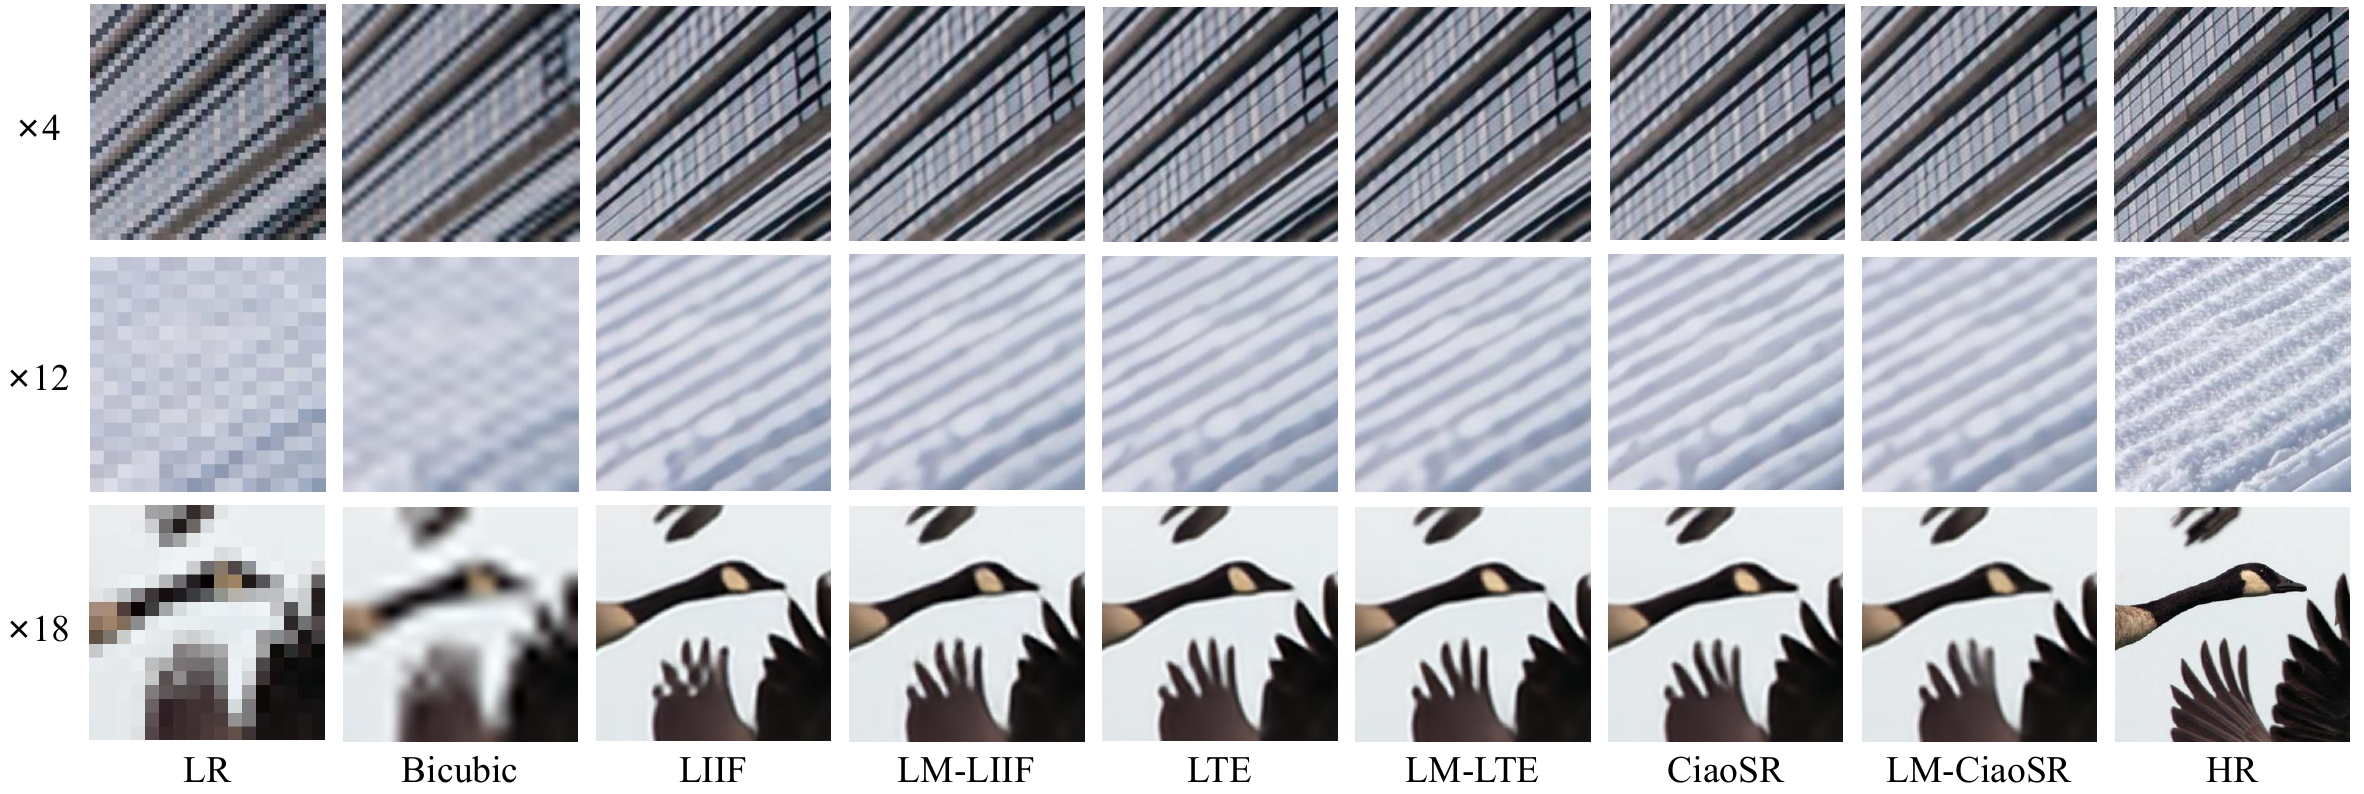}
  \caption{Qualitative comparison for ASSR. All of the ASSR methods use RDN as the encoder.}
  %\Description{}
  \label{fig:qualitative_comparison_rdn}
\end{figure*}
